# Supplementary material for: RoboGene: Diversity-Driven Agentic Task Generation Framework for VLA Pre-training
Source: arXiv:2602.16444 source file (2026-10-26)
Supplement: Supplementary file 1 [file ijcai26_supp.tex]

\typeout{IJCAI--ECAI 26 Instructions for Authors}

\documentclass{article}
\pdfpagewidth=8.5in
\pdfpageheight=11in

\usepackage{ijcai26}

\usepackage{times}
\usepackage{soul}
\usepackage{url}
\usepackage[hidelinks]{hyperref}
\usepackage[utf8]{inputenc}
\usepackage[small]{caption}
\usepackage{graphicx}
\usepackage{amsmath}
\usepackage{amsthm}
\usepackage{booktabs}
\usepackage{algorithm}
\usepackage{algorithmic}
\usepackage[switch]{lineno}

\linenumbers

\urlstyle{same}

\pdfinfo{
/TemplateVersion (IJCAI.2026.0)
}

\input{0-macro.tex}

\title{\LARGE \bf
RoboGene: Boosting VLA Pre-training via Diversity-Driven Agentic Framework for Real-World Task Generation
}

\author{
    Supplementary Material
}

\iffalse
\author{
First Author$^1$
\and
Second Author$^2$\and
Third Author$^{2,3}$\And
Fourth Author$^4$\\
\affiliations
$^1$First Affiliation\\
$^2$Second Affiliation\\
$^3$Third Affiliation\\
$^4$Fourth Affiliation\\
\emails
\{first, second\}@example.com,
third@other.example.com,
fourth@example.com
}
\fi

\begin{document}

\maketitle

\appendix

\input{supp/7-appendix}

{
\small
\bibliographystyle{named}
\bibliography{ijcai26}
}

\end{document}
